# Supplementary material for: Unsupervised Numerical Reasoning to Extract Phenotypes from Clinical Text by Leveraging External Knowledge
Source: arXiv:2204.10202 source file (2022-04-19)
Supplement: Supplementary file 1 [file appendix.tex]

\section{Appendix}
